# Supplementary material for: Remember When It Matters: Proactive Memory Agent for Long-Horizon Agents
Source: arXiv:2607.08716 source file (2026-07-09)
Supplement: Supplementary file 1 [file 8_appendix.tex]

\input{sections/2_related}
